# Supplementary material for: Creating a Domain-diverse Corpus for Theory-based Argument Quality Assessment
Source: arXiv:2011.01589 source file (2020-11-03)
Supplement: Supplementary file 1 [file debate_gl.pdf]

# Overview: help us judge argument quality

The goal of this task is to evaluate the argumentative quality of informal text. You will first decide whether a given text is argumentative or not. For texts you find argumentative, you will score each of three traits: **cogency**, **effectiveness**, and **reasonableness**. You will then assign an **overall** score for the entire text snippet.

## What we provide:

Each passage presented to you will have a title containing the topic of discussion. Some titles will explicitly state the author's stance on the topic. Although some titles contain a stance, this does not guarantee that the passage is argumentative (see *Judging argumentativeness*). The texts are from online debate forums in which users discuss a wide variety of controversial topics.

# Steps

1. Read the given title and passage.
2. Decide if the passage is argumentative.
    1. If you are unable to objectively judge the example, please choose the option that reflects why.
        - Use 'This text is not readable' only if you are not able to read and understand the example (e.g., the text is gibberish or in another language).
        - Use 'I cannot provide an objective judgment' only if your personal bias makes it impossible for you to tell if the example is argumentative and objectively score it.
    2. If you decide that the text is not argumentative, click the 'No' option and move to the next example.
    3. If you decide that the text is argumentative, click the 'Yes' option.
3. You will evaluate three traits for each text: a) cogency, b) effectiveness, and c) reasonableness.
    1. For each trait, ***mentally*** answer each of the questions presented to you with 'yes' or 'no'.
    2. Provide a score for each trait based off of your answers-- a 'yes' answer raises the score and a 'no' answer lowers it. You will score each trait on a 5-point scale:

       1: Very Low - 2: Low - 3: Medium - 4: High - 5: Very High
       **Note that the number of questions is not necessarily aligned with the scale.**

**Your answers should loosely inform your scoring.**

3. Score the overall quality of the argument last.
4. Move to the next example.

## Notes:

1. Try to be as objective as possible. Whether or not you agree with the author **should not influence** whether you think the example is argumentative or how you score the example.
2. Some of the opinions stated may be offensive. If you are too offended by an example to provide an objective judgment, please choose 'I cannot provide an objective judgment' and skip to the next instance.
3. Assume the **target audience** consists of adult internet users who are open-minded, non-hostile, receptive, and generally open to being persuaded.
4. **Remember to submit your work and close the window if you are going to step away from the task for a period of time.**

# Judging argumentativeness

A text should be seen as argumentative if it conveys the author's claim on an issue and the author is arguing for their claim. A text is not argumentative if it states the author's opinion on a topic without any justification for their opinion. To be considered argumentative, a text must contain a claim and a justification.

**Note: A text is argumentative if the author argues for a claim, even if they only provide one reason for their belief.**

**Note: If the title contains a claim but the passage does not, consider if the passage provides a justification for the claim in the title. If so, the passage is considered argumentative.**

**Examples: Judging argumentativeness**

→ Claims are in orange, Justifications are in green

| Argumentative? | Text | Reason |
|---|---|---|

| | | |
|---|---|---|
| **Yes** | (*Hypothetical example*)<br><br>You have to eat your vegetables because I said so. | The author makes a claim and provides a justification for that claim. This passage is an argument, even though it is weak. |
| **Yes** | (*Hypothetical example*)<br><br>**Title:** Cherry candy is the best<br><br>**Passage:** Because I like it. | Though the *passage* does not contain a claim, the *title* contains a claim. The passage includes a justification for this claim. This passage is an argument, even though it is weak. |
| **Yes** | **Title:** CMV: Americans don't actually like turkey on Thanksgiving, but eat it out of tradition.<br><br>**Passage:** When will America really face the hard truth? Turkey is overrated. I don't care how "moist" your gram-gram makes it. Bake it. Fry it. It's a dry ass bird. You work on it forever in your mouth till it forms that familiar turkey paste you have to choke down every year. If we really loved turkey, there would be a successful chain of Turkey based restaurants. We don't. We keep lying to ourselves, while we fill up on everything but turkey. Leftovers? Mostly turkey. A dozen people can't eat a whole bird? I've seen less eat a whole pig! Fuck turkey! Stop the madness! | The author's claim is clear and they argue for their claim by listing reasons for their belief. |
| **No** | **Title:** banning plastic water bottles; Stance: No<br><br>**Passage:** Yeah I have a bottle of water next to me its no bid deal! | The author expresses a claim ("its no bid deal") but does not argue for their claim. |
| **No** | **Title:** gay marriage right or wrong; Stance: allowing gay marriage is right<br><br>**Passage:** The"'who gives a crap" button was your browser's back button. No one said you had to read this or vote on this or post a comment. It always baffles me to see people take the time to post a comment to say they don't care and everyone should stop talking about it. And | This comment is off-topic and corresponds more to an emotional outreach. The author neither presents their opinion nor argues for it. |

| | | |
|---|---|---|
| | another thing... people who post comments like mine make me sick. | |
| **Yes** | **Title:** CMV: Universities That Accept Public Money Should Be Required To Follow Constitutional Amendments<br><br>**Passage:** Public universities to0 often disregard first amendment freedoms by setting up freedom of speech zones and strict student handbook codes. They created these because they were overly concerned with people becoming offended. This goes against what higher education was created for and nullifies their role as a sounding board for ideas and change.<br><br>* The problem is such an issue organizations like the Foundation For Individual Rights In Education have been created<br><br>* The Christian organization Alliance Defending Freedom has responded to many college campus speech violations in the last few years<br><br>We need to tackle this trend before it becomes more commonplace then it already is. | The author clearly states their claim and then lists why they believe this is a problem. |
| **No** | **Title:** CMV: I want to move very far away for college while my parents want me to stay local/in-state.<br><br>**Passage:** There are a few things I need to touch on; first and probably most important, I come from a family of means so while tuition is a factor it isn't going to be the sole purpose of the school that I'll be attending. Second to give you perspective I live in the American Northeast and I want to go far west to a university in states such as Nevada, Arizona, and Colorado. And lastly this post isn't going to be the deciding factor of where I'm going to school, I just want to see the other side of the argument. | The author does not provide reasons for their claim and is just asking for others' opinions. |

# Judging argument quality

We've chosen to break the quality of an argument into the three traits listed below. You should refer to these definitions when scoring each trait.

## **Cogency:** The argument includes acceptable justifications that are relevant to the point the author is making and that are sufficient to draw the author's conclusion.

Considering only the **individual justifications for the author's claim**, answer each of the following questions before scoring cogency:

- Are the justifications for the argument acceptable/believable?
- Are the justifications relevant to the author's point?
- Do the justifications provide enough support to draw a conclusion?

A 'yes' answer to each of these questions should increase the cogency score and 'no' should lower it.

**Examples: Scoring cogency**

→ Claims are in orange, Justifications are in green

| Score | Text | Reason |
|---|---|---|
| **5: Very High** | **Title:** should physical education be mandatory in schools; Stance: yes<br><br>**Passage:** Most people think that PE classes are completely useless because the only thing you would normally do in a PE class is run around. But there is more to a PE class then just running around the field for an hour. With physical education you can get muscles, you can become stronger, it wouldn't be so easily for you to become fat (of course you would also need to keep a balanced diet) and for further ages (like 60-80) it would prevent you from having heart attacks. With the help of this class there would be fewer obese children around the globe and more fit and strong people. | The author provides justification for their claim. The reasons presented are believable, relevant, and sufficient in drawing a conclusion. |

| | | |
|---|---|---|
| **4: High** | **Title:** firefox vs internet explorer; Stance: it has a cute logo oh and extensions err add ons<br><br>**Passage:** firefox is much better.<br><br>It remembers passwords with greater gusto.<br><br>add-ons allow you to personalize your browser in every way. I love - tabs (aging and remembering them when you close the browser, weatherfox, gestures,<br><br>there is even a tab that lets you display the page in IE format if something is incompatible (rare, only SAP at work)<br><br>and the way you can put the link logos in the tool bar rocks.<br><br>much friendlier and a better browser, and not just because i don't want to support MS. Because i don't care about that, a good product is a good product. | The author provides justification for their claim. The reasons presented are believable, relevant, and may or may not be sufficient in drawing a conclusion. |
| **3: Medium** | **Title:** CMV: people like al sharpton, Facebook SJWs and the media love to rally around cases where they know they are wrong- because their goal is not justice, it's attention for themselves.<br><br>**Passage:** I know there is a problem with how the cops treat black people. But why are the cases that are most blasted over the media only focused on thugs?<br><br>There are real cases of mistreatment out there. Cory Maye is one I learned about here on reddit today. Where are the Facebook sjw assholes and people like sharpton for a case like that? The only stories I found about maye were on huffpo. How is that possible??<br><br>I now believe the media, sjw assholes, and people like sharpton are in this solely to get attention for themselves. They purposely pick cases to champion where they can see how they're wrong, because the goal isn't change, it's attention for themselves. And in the end they only hurt their supposed cause. | The author presents support for their point but not enough to draw a conclusion |

| | | |
|---|---|---|
| **2: Low** | **Title:** Is anything in this world free?-- Stance: Nothing in this world is free.<br><br>**Passage:** The Way I see it is that nothing in this world is truly free. There will always be a cost for everything. Even Freedom in not free, because it too has its opportunity costs. Oxygen is not free because it uses up energy same thing with dying even existence uses up energy. Thus nothing in this world is free because we must first give something of equal or greater value to obtain what we wish for. | Though the author makes relevant points, they may or may not be acceptable and are not backed by a sufficient amount of evidence. |
| **1: Very Low** | **Title:** gay marriage right or wrong; Stance: allowing gay marriage is wrong<br><br>**Passage:** Of course its wrong.<br><br>Why do you think Aids exists? | The author provides no justification for their claim. |

**Effectiveness:** The way the argument is presented persuades you to agree with the author, e.g. the author changed your mind or affirmed a point you already agreed with.

Answer the following questions before scoring effectiveness:

- Is the author qualified to be making the argument? Assume yes unless you have reason to believe the author is lying or otherwise should not be believed.
- Does the argument evoke emotions that make the audience more likely to agree with the author?
- Does the author's language make it easy for you to understand what they are arguing for or against? Does the author use grammatically correct and unambiguous language? Do they avoid unnecessary complexity and stay on topic?
- Is the author's argument and delivery appropriate for an online forum? (Note: Offensive language should always be considered inappropriate.)
- Did the author present their argument in an order that makes sense?

A 'yes' answer to each of these questions should increase the effectiveness score and 'no' should lower it.

**Examples: Scoring effectiveness**

→ Claims are in orange, Justifications are in green

| Score | Text | Reason |
|---|---|---|
| **5: Very High** | **Title:** if your spouse committed murder and he or she confided in you would you turn them in; Stance: yes<br><br>**Passage:** As an ambitious, young person wanting to become a lawful, successful, homicide detective, I would not be lenient with any murderer in my midst. Hopefully, the murder wouldn't be the result of a pleasure/malicious-kill, so that the sentencing won't be as harsh, but nonetheless, all murderers must be tried. After all, hopefully my spouse will understand that having to live in hiding is basically the same as being in prison except much worse since there would be little chance for parole since they will have to live with the guilt and/or the fear of being caught for the rest of their lives. | The author presents their argument using clear organization and language. The author states their opinion and then presents supporting points, which is an effective organizational structure. The author is explicitly qualified to be making the argument and increases emotional appeal by personally relating to the topic. |
| **4: High** | **Title:** is the school uniform a good or bad idea; Stance: bad<br><br>**Passage:** The school my mother works at, plus the school district my cousin's 3 children are in, are utilizing school uniforms. One reason is to "reduce bullying", which in reality, doesn't even address the problem concerning bullying. The only good it does is that it gets rid of or reduces students being bullied because they aren't wearing a specific clothing label that they dictate is the IN thing to wear. While it's a problem, all it does is sweep the one basic type of bullying under the rug. Kids will find other reasons to bully others. It also infringes upon their basic rights to be individuals and to express their individuality. | The author presents their argument using clear organization and language. The author presents the argument using an organized structure. The argument is lacking in emotional appeal. |

| | | |
|---|---|---|
| **3: Medium** | **Title:** firefox vs internet explorer; Stance: it has a cute logo oh and extensions err add ons<br><br>**Passage:** Firefox takes the best of all previous browsers and sticks it all in one neat package. Security and extendibility are some of its top features. And those times when FF seems to eat up a lot of memory? That's just the cache so you're able to surf the net even faster. Just lower the cache if you don't want to eat so much memory. | Although the argument is appropriate, the author does not evoke an emotional response. The organization of the argument could be improved. |
| **2: Low** | **Title:** christianity or atheism; Stance: atheism<br><br>**Passage:** Religion in the past has caused many wars. It encourages racism , sexism and homophobia. It is something that gives us prejudice. It makes us hate one another. the time has come to put a stop to it. | The author does not evoke an emotional response that makes the argument more agreeable. The argument's organization could be improved. |
| **1: Very Low** | **Title:** is porn wrong; Stance: yes porn is wrong<br><br>**Passage:** well, the people who watch porn,i guess thats ok, its NORMAL. but the people who areIN the porn, that is not normal..i read it in a abnormal psychology book,that means they have a disorder | The way the argument is written and organized is hard to follow. The offensive nature is not appropriate for an online forum. |

**Reasonableness:** The argument contributes to the resolution of the given issue in a sufficient way that is acceptable to the target audience.

Considering the **entire argument**, answer the following questions before scoring reasonableness:

- Would the target audience accept the argument and the way it is stated?
- Would the target audience judge the argument as worthy of being mentioned in the larger discussion?
- Does the argument contribute to the resolution of the given issue? Does it provide information that helps the audience arrive at a conclusion?

- Does the argument address and adequately rebut counterarguments?

A ‘yes’ answer to each of these questions should increase the reasonableness score and ‘no’ should lower it.

**Note:** You should be open to seeing an argument as relevant even if it does not match your stance on the issue. Do not judge based on whether or not you agree with the author. Instead, **judge from the perspective of the target audience (see *Note 3*)**.

**Examples: Scoring reasonableness**

→ Claims are in orange, Justifications are in green

| Score | Text | Reason |
|---|---|---|
| **5: Very High** | **Title:** if your spouse committed murder and he or she confided in you would you turn them in; Stance: yes<br><br>**Passage:** As an ambitious, young person wanting to become a lawful, successful, homicide detective, I would not be lenient with any murderer in my midst. Hopefully, the murder wouldn't be the result of a pleasure/malicious-kill, so that the sentencing won't be as harsh, but nonetheless, all murderers must be tried. After all, hopefully my spouse will understand that having to live in hiding is basically the same as being in prison except much worse since there would be little chance for parole since they will have to live with the guilt and/or the fear of being caught for the rest of their lives. | The target audience would consider the argument valid and worthy of being considered in the larger discussion. The author provides information that helps the audience arrive at a conclusion. |
| **4: High** | **Title:** is the school uniform a good or bad idea; Stance: bad<br><br>**Passage:** The school my mother works at, plus the school district my cousin's 3 children are in, are utilizing school uniforms. One reason is to "reduce bullying", which in reality, doesn't even address the problem concerning bullying. The only good it does is that it gets rid of or reduces students being bullied because they aren't wearing a specific clothing label that they dictate is the IN thing to wear. While it's a problem, all it does is sweep the one basic type of bullying under the rug. Kids will find other reasons to bully others. It also infringes upon their basic rights to be individuals and to express their individuality. | The author addresses counterarguments. The target audience may not accept the way the argument is stated because it makes broad generalizations. |

| | | |
|---|---|---|
| **3: Medium** | **Title:** india has the potential to lead the world; Stance: no against<br><br>**Passage:** All we can say is a big IF because we are not yet 100% sure if this nation itself could lead the whole world. Who knows maybe in the future that India could fail to lead us. There are still other countries who are more progressive, more literated, more powerful than India, like the USA, United Kingdom, Russia, Japan, etc. This nation doesn't have yet enought potentials and ability to sustain the needs of the people. India is not yet that full of technologies like in the Americas. Well in fact technology is one of the most sophisticated and essential inventions ever created. | The argument presents some information that contributes to the discussion but does not address counterarguments. |
| **2: Low** | **Title:** christianity or atheism; Stance: atheism<br><br>**Passage:** No one ever said science is PERFECT. That's the difference between Religion and Science, Science admits it doesn't have all the answers while Religion is SO dogmatic enough to not even recognise FACTS. And even just what TRUTH really stands for. | The author does not provide information that supports the argument and thus does not contribute to the larger discussion. Counterarguments are not addressed. |
| **1: Very Low** | **Title:** should physical education be mandatory in schools; Stance: no<br><br>**Passage:** Gym class is a useless class that students waste time in. There should be a test and if people can not run a mile without stopping every couple feet they should join. There is also the fact people can join to get prepared for sports. Students should have that class time to use it towards their careers and not a class that is just there. | The author does not contribute to the resolution of the issue and does not address counterarguments. |

**Overall:** Judge the overall quality based on your ratings of cogency, effectiveness, and reasonableness. Also, take anything outside of these three traits that influences argument quality into account.

**Note: The scores for cogency, effectiveness, and reasonableness should inform the score you give for overall quality. Therefore, overall quality should be judged after each of the three traits above.**

**Examples: Scoring overall**

→ Claims are in orange, Justifications are in green

| Score | Text | Reason |
|---|---|---|
| 5: Very High | **Title:** india has the potential to lead the world; Stance: yes for<br><br>**Passage:** The Indian economy is galloping at a breakneck speed and might even reach double-digit growth by 2013, feel Finance Minister Pranab Mukherjee and Commerce Minister Anand Sharma. Many economists agree that the demographic dividend that India enjoys could see the country sustain its high growth rate for a long time to come. The India growth story is indeed enviable. Despite being plagued by myriad problems, India has emerged stronger and more resilient to any global crises so far. India is expected to be the world's fastest growing economy by 2018, according to Economist Intelligence Unit, a research arm of the Economist magazine. | The argument presents support that is believable, reasonable, and appropriate for the topic. The author addresses counterarguments and cites credible sources. |
| 4: High | **Title:** is it better to have a lousy father or to be fatherless; Stance: fatherless<br><br>**Passage:** It really sucks not having a man to look up to while your growing up. I believe that being fatherless is better then having a lousy father. The reason I believe this is the best is because you dont want to be looking up to a guy that does nothing in life and its just setting bad examples. Who knows you might grow up following his steps. So being fatherless is better because from day one you start depending on your own with no need of a father being there. And theres always going to be other people by your side helping you get through life. | The author supports their claim with appropriate justifications and addresses counterarguments. |
| 3: Medium | **Title:** should physical education be mandatory in schools; Stance: no<br><br>**Passage:** OK no and yes I think p.e should be education which is teaching students how to eat right and live a healthy life style not making a fat kid run 10 laps around a track but showing them that eating right and exercise can BE FUN not having an obese child being bully because they can't run as fast as someone else. That is what physical education could be real EDUCATION. Students should not feel bad if they can't run a 5k or do 20 push ups. | The argument evokes an emotional response but is not presented in an organized manner. |

| | | |
|---|---|---|
| **2: Low** | **Title:** india has the potential to lead the world; Stance: no against<br><br>**Passage:** i think, the india is not ready to lead the world because of many reasons..<br><br>1.) the politians of our country are involved in black money cases. they try to gain or earn money as possible.<br><br>2.) they always try to make a big issue of useless topics. e.g., if a politian says something about another politian, they try to make it a big issue . | The argument does provide evidence for its claims but may not be considered in the resolution of the issue. |
| **1: Very Low** | **Title:** gay marriage right or wrong; Stance: allowing gay marriage is wrong<br><br>**Passage:** gays are overrated. it is another "look at me" stunt. i think gays are the product of overly protective parents, abuse, or liberal wakoness (it should be a disease).if you gays would stop calling attention to yourselves, nobody would really care what you do. | The argument is not supported, does not contribute to a resolution of the issue, and would not be considered worthy of being mentioned by the target audience. |
