# Supplementary material for: Creating a Domain-diverse Corpus for Theory-based Argument Quality Assessment
Source: arXiv:2011.01589 source file (2020-11-03)
Supplement: Supplementary file 2 [file yahoo_gl.pdf]

# Overview: help us judge argument quality

The goal of this task is to evaluate the argumentative quality of answers from Yahoo Answers. In this forum, an original poster (OP) posts a question, which is answered by a member of the community. The goal of this task is to evaluate the quality of arguments made **in the answers**.

You will first decide whether a given answer is argumentative or not. For answers you find argumentative, you will score each of three traits: **cogency**, **effectiveness**, and **reasonableness**. You will then assign an **overall** score for the entire text snippet.

## What we provide:

- **Question:** A question from the OP
- **Context:** A short text written by the OP that explains the question
  - Not all questions include a context.
- **Answer:** An answer to the question provided by another user

For each example, you will judge the argumentative quality of the **answer** provided. The question and context indicate the topic of discussion and are provided for context.

# Steps

1. Read the given question and answer. Read the context if it is provided.
2. Decide if the **answer** is argumentative.
   1. If you are unable to objectively judge the answer, please choose the option that reflects why.
      - Use ‘This text is not readable’ only if you are not able to read and understand the example (e.g., the text is gibberish or in another language).
      - Use ‘I cannot provide an objective judgment’ only if your personal bias makes it impossible for you to tell if the example is argumentative and objectively score it.
   2. If you decide that the answer is not argumentative, click the ‘No’ option and move to the next example.
   3. If you decide that the answer is argumentative, click the ‘Yes’ option.
3. You will evaluate three traits for each text: a) cogency, b) effectiveness, and c) reasonableness.
   1. For each trait, mentally answer each of the questions presented to you with 'yes' or 'no'.

2. Provide a score for each trait based off of your answers-- a ‘yes’ answer raises the score and a ‘no’ answer lowers it. You will score each trait on a 5-point scale:

   1: Very Low - 2: Low - 3: Medium - 4: High - 5: Very High
   **Note that the number of questions is not necessarily aligned with the scale. Your answers should loosely inform your scoring.**

3. Score the overall quality of the argument last.

4. Move to the next example.

### Notes:

1. Try to be as objective as possible. Whether or not you agree with the author **should not influence** whether you think the example is argumentative or how you score the example.
2. Some of the opinions stated may be offensive. If you are too offended by an example to provide an objective judgment, please choose ‘I cannot provide an objective judgment’ and skip to the next instance.
3. The **target audience** refers to forum users who are interested in the given question. Assume this group consists of adult internet users who are open-minded, non-hostile, and receptive.
4. Some arguments are old and may be dated. This should not affect how you score the example.
5. Remember to submit your work and close the window if you are going to step away from the task for a period of time.

### Tips

1. After you score a trait, collapse the trait's questions by clicking on the gray box with the trait name. This makes it easier to read the passage while judging the next trait.

# How to judge argumentativeness

An answer should be seen as argumentative if it conveys the author’s claim on an issue and the author is arguing for their claim. An answer is not argumentative if it states the author’s opinion on a topic without any justification for their opinion. To be considered argumentative, a text must contain a claim and a justification.

Note: A text is argumentative if the author argues for a claim, even if they only provide one reason for their belief.

### How to judge advice

Some answers give advice or factual information to the original poster. These types of answers are argumentative if the author states a claim or opinion with a reason why. If the answer says 'I think' or 'I believe,' this is a sign that the answer is argumentative. For example:

**Question**: If a person split 100 acres between 2 sons with a living interest but his will says executor gets 10%?

**Answer**: First, the "life interest" you refer to is called a life estate. It means that the son gets the acres for his lifetime and upon death the land passes to whomever was designated as the remainderman or else it reverts back to the grantors estate. As for your question, I think because the man passed the property as an inter vivos gift (ie, outside the will), any provision in the will giving the property away to the executor would be void. the legal doctrine is called ademption by extinction.

→ This answer is argumentative because it states the author's opinion on a legal matter along with a reason for their opinion.

**Question**: What do you do if your hunting camp is burglarized and you don't know who the culprit was?

**Answer**: Cry over what was stolen, then go and replace all the stuff that was stolen because the police will not find your stuff for you. They will tell you, " If anything turns up we will let you know." Yeah Right. Do like I did, purchase a truck that I put a topper with a locking door on it and I added another 2 locks to the topper to keep honest people out. It has worked for me so far.

→ The answer is argumentative because it gives advice to the user. The author provides a reason for their advice.

**Examples: Judging argumentativeness**

→ Claims are in orange, Justifications are in green

| Text | Argumentative? | Reason |
| --- | --- | --- |

| | | |
|---|---|---|
| **Question:** Being sued , what happends if i dont pay?<br><br>**Answer:** Stocko's generally right regarding what happens if you don't pay. Having an unpaid civil judgment will haunt you everywhere you go, from credit to job applications. You may be forced into involuntary bankruptcy. DO NOT let a default happen. Get an attorney, or at least proceed "pro se" (without an attorney) and answer any lawsuit. Because the insurance company knows you're not represented and didn't have insurance, they're going to go at you hard. Merely getting a lawyer (if you can afford $1-2,000) should help this settle quickly. | **Yes** | The author makes a claim about how the original poster should handle a situation. The author presents reasons for the advice that they give. |
| **Question:** what is the differnce between a rigid and a flexible constitution?<br><br>**Answer:** Are you asking "living document?" as opposed to a document meant to be applied by original intent?<br>Original intent assumes one has studied the debates and opinion of the writers of the Constitution and applies that logic, allowing changes through proper course.<br>Living document assumes you either "know" what the authors would have agreed upon today or more correctly what YOU want the Constitution to say, therefore by YOURInterpretation…That's what it says. | **No** | The author is just giving information and not making a claim. |
| **Question:** Do you think servers should be paid more than $2.13 and hour?<br><br>**Answer:** I've never been a server or waitress but, I feel that regardless of how much in tips they make, they should get minimum wage. They work just as hard as anyone else. As for the tips, they have to earn them. Just think of a slow night and little or no tips...she walks away with what, 20 bucks for working 8 hours on her feet. I think there should be a change in this, everyone should get nothing less than minimum wage regardless of their occupation. | **Yes** | The author makes the claim that 'they should get minimum wage'. They then argue for their claim by stating justifications for their claim. |

| | | |
|---|---|---|
| **Question:** I was at a Party where the host invited us to smoke cigars on the porch. Naturally the conversation turned?<br><br>**Answer:** until just before the band. on the tip of the cigar should be a "crown". a small piece of wrapping to secure the cigar. you should be able to see it if you look very closely. looks almost like a leaf cap on the end. cut it just above the bottom of the cap. cutting it all off might unravel the cigar. this only applies if you're using guillotine snips. if you're using a v cut snip then it doesn't matter. | **No** | There is no claim stated in the text. The author is telling a story, not arguing for a claim. |
| **Question:** what's the difference between a regular lawsuit or class action lawsuit?<br><br>**Answer:** In a class action law suit, you are in a large group of people who were victims of a faulty or dangerous product on the market such as a car or a bad drug that caused you to get very sick or end up dead. You split the award(s) with everyone else. BUT the lawyers make the most money out of that deal and you end up getting a very small amount of $$$ after all is said and done. The good part is that you don't have to give a private attorney a large cut of the award yourself in a private civil suit. Either way, you don't really get the full amount you truly deserve.<br><br>Lawyers are crooks!! | **Yes** | The author makes the claim that “lawyers are crooks” based on the justifications listed. |

# How to judge argument quality

We’ve chosen to break the quality of an argument into the three traits listed below. You should refer to these definitions when scoring each trait.

**Cogency:** The answer includes acceptable justifications that are relevant to the point the author is making and that are sufficient to draw the author’s conclusion.

Considering only the **individual justifications for the author's claim**, answer each of the following questions before scoring cogency:

- Are the justifications for the argument acceptable/believable?
- Are the justifications relevant to the author’s point?

- Do the justifications provide enough support to draw a conclusion?

A ‘yes’ answer to each of these questions should increase the cogency score and ‘no’ should lower it.

**Examples: Scoring cogency**

→ Claims are in orange, Justifications are in green

| Text | Score | Reason |
|---|---|---|
| **Question:** how come Asians can't drive?<br><br>**Answer:** It's not a matter of Asians, but of how accustomed to motor vehicle operation the driver is.<br><br>A New Yorker who didn't operate a car until they were 30, and moved to California, won't be a very experienced driver, and therefore not very good at it.<br><br>Likewise, anyone who is very new to driving will seem a little clumsy. Since mass amounts of cars like we have in the Western world are still not quite commonplace in Asia, you'll see this syndrome with folks from these areas who haven't operated a car until they got here.<br><br>The question is one of experience behind the wheel, and not necessarily one of ethnicity. | **5: Very High** | The answer contains acceptable and believable justifications for the author’s claim. The justifications are relevant to the author’s point and are sufficient in drawing a conclusion. |
| **Question:** Is the use of the Internet making a diffrence in the way our lives are organized? What really has changed?<br><br>**Answer:** The Internet has made the world much smaller. It has changed the way we operate in our daily lives as well as in business. A recent example of how the Internet affects even the most destitute of people would be the use of notebooks and the Internet by caseworkers with Adult Protective Services in Texas. The technology they have recently introduced is awesome. A caseworker can pull up all the information needed on a client from just about anywhere. When in the home, he/she can complete most all of the documentation. If they get lost, all they have to do is access the | **4: High** | The argument includes acceptable and relevant justifications that may or may not provide enough support to draw a conclusion. |

| | | |
|---|---|---|
| Internet and Yahoo Maps. It has really streamlined their work. | | |
| **Question:** My "friends" are trying to get me to smoke pot and say it doesn't hurt you. Is that true?<br><br>**Answer:** Well, it sounds like you don't really consider them "friends," and therefore you should not let them convince you to do something you don't want to do. In fact, you shouldn't let anyone do that. As far as pot being harmful to you, I imagine that if you were responsible when using it, it would not greatly affect your health. Much like being responsible when drinking alcohol. However, it is illegal, so you do want to take that into consideration. | **3: Medium** | The author provides some relevant and acceptable justifications for their claim but not enough to draw a conclusion. |
| **Question:** what's the difference between a regular lawsuit or class action lawsuit?<br><br>**Answer:** In a class action law suit, you are in a large group of people who were victims of a faulty or dangerous product on the market such as a car or a bad drug that caused you to get very sick or end up dead. You split the award(s) with everyone else. BUT the lawyers make the most money out of that deal and you end up getting a very small amount of $$$ after all is said and done. The good part is that you don't have to give a private attorney a large cut of the award yourself in a private civil suit. Either way, you don't really get the full amount you truly deserve.<br><br>Lawyers are crooks!! | **2: Low** | The justifications for the author's claim may not be believable or provide enough support to draw a conclusion. |
| **Question:** Hi All;) What is 'deja vu' exactly, and what explanations are out there?) ...See details:)?<br><br>**Answer:** I always heard that deja vu occurs from a mis-firing of the brain. Instead of what is currently happening going to your short term memory and then to your long term memory, the reverse happens. This is why you think of the event of a memory, or of already having | **1: Very Low** | The justifications for the author's claim are not believable. |

| | | |
|---|---|---|
| happened. I don't have a source for this, it just makes sense to me. | | |

**Effectiveness:** The way the answer is presented persuades you to agree with the author, e.g. the author changed your mind or affirmed a point you already agreed with.

Answer the following questions before scoring effectiveness:

- Is the author qualified to be making the argument? Assume yes unless you have reason to believe the author is lying or otherwise should not be believed.
- Does the argument evoke emotions that make the audience more likely to agree with the author?
- Does the author's language make it easy for you to understand what they are arguing for or against? Consider if the author uses grammatically correct and unambiguous language, avoids unnecessary complexity, and stays on topic.
- Is the author's argument and delivery appropriate for an online forum? (Note: Offensive language should always be considered inappropriate.)
- Did the author present their argument in an order that makes sense?

A 'yes' answer to each of these questions should increase the effectiveness score and 'no' should lower it.

**Examples: Scoring effectiveness**

| Text | Score | Reason |
|---|---|---|
| **Question:** Disadvantages of nuclear family?<br><br>**Answer:** Compared to an extended family, A LOT. If one of the immediate family members disagree with each other on fundamental issues, that's it, the whole structure will crumble and you have a broken family and the kids will have no relatives to run to for support. I mean, they may have relatives but they will not be close enough for them to feel comfortable just knocking on their door.<br><br>Holidays are boring. You'll get cabin fever more often and... well, it's just lonely. Bigger families are more fun. | **5: Very High** | The answer is appropriate for the domain and is presented in a sensical order. The author evokes emotions that make the argument more agreeable. The author's language makes it clear what they are arguing for. |

| | | |
|---|---|---|
| **Question:** Any tips on how to not waste time?<br><br>**Answer:** don't do online things like yahoo! answers. heh heh..<br><br>more seriously... you have to be motivated. You have to have a heartfelt reason for why you would want to sacrifice leisure activities to maintain focus. If the reason isn't better than the reward you get for being lazy, then it will be very difficult to stay on track.<br><br>For instance, let's say you want to study everyday instead of waiting until last minute. One way to stay on task is to realize that the habit of studying daily will help you in graduate school. And you want to get that doctorate because you would be the first in your family to do so and that would make you very happy.<br><br>If the reason doesn't make you happier than being lazy, you'll never stay focused.<br><br>Sometimes even negative reasons help to motivate (although it may not be psychologically healthy). Like you really would like to show all those people you really hate that you're better than them. That would work too. | **4: High** | The author uses clear and appropriate language and structures their argument in a way that makes sense. The answer evokes an emotional response. |
| **Question:** Would legalisation of gay marriage have a negative effect on society??<br><br>**Answer:** If it had any negative effect, it would be less than the effect of making divorces so easy. The disposable marriage has done far more damage to our society than legalizing gay marriage.<br><br>For all those who want to compare the current laws against gay marriage to illegalizing bi-racial marriage, I'd like to point out that the definition of marriage allows specifies man & woman. But that doesn't mean we can't redefine marriage to include same sex couples.<br><br>I would support a bill allowing gay marriage here in Texas, but I have sympathy for those who feel differently. I came from a very conservative family (My mom thought the Baptist were | **3: Medium** | The author personally relates to those who have the opposite view, which makes the argument more agreeable and is appropriate for the domain. The language and ordering of the argument does not make it very clear what the author is arguing for. |

| | | |
|---|---|---|
| liberals) but I am more of a libertarian now. So I've seen life from both perspectives. What the conservatives don't seem to get is that just because they believe something is wrong, that doesn't neccesarily mean it should be illegalized. | | |
| **Question:** Is it illegal to purchase cigarettes online from a different state?<br><br>**Context:** I have found cheap(er) cigarettes online (I live in NYC). Is it legal to purchase from these sites? It would let me, but I have been afraid to press "Send" on the order!<br><br>**Answer:** It is not illegal to buy cigarettes online from a diffeent state. It IS illegal to fail to pay New York State and City cigarette sales tax on those cigarettes. You should buy the cigarettes online, compute the tax on the cigarettes and mail it to the city and state. Otherwise, you are breaking the law.<br><br>But, of course, what you should really do is what New York City wanted you to do when they raised the tax in the first place - quit smoking. One half of all people who smoke will die from it. | **2: Low** | The answer evokes emotions that make the audience less likely to agree with the author in that the author is telling the original poster what to do. The author is not necessarily qualified to give advice and this is not appropriate given the question. |
| **Question:** How come we have abortion is legal but not the right to die?<br><br>**Context:** Why do we live in a society where we can't choose to end our own lives but we can choose to prohibt the life of another from existing?<br><br>Don't get me wrong, I'm not trying to start the whole pro-life or pro-chooice debate, I just want to know why we can't kill ourselves legally....<br><br>**Answer:** Very good question!!!! My nephew was 28 wks at birth and he died, he was a whole little man. All his fingers and toes, etc. and it is legal to abort at this stage in LIFE.<br><br>And if my pet is suffering I can have them put to sleep. | **1: Very Low** | The language of the answer makes it hard to tell what the author is arguing for. Their argument is not presented in a sensical order. |

| | | |
|---|---|---|
| But I am forced to watch a loved one die because we can't even do for them as we would a pet!!!!!! Hmmmmmm<br><br>OUR GOVERNMENT????????? | | |

**Reasonableness:** The answer sufficiently contributes to the resolution of the question in a way that is acceptable to the target audience.

Considering the **entire answer**, answer the following questions before scoring reasonableness:

- Would the target audience accept the argument and the way it is stated?
- Would the target audience judge the argument as worthy of being considered in answering the question?
- Does the argument address and answer the question? Does it provide information that helps the audience arrive at a conclusion?
- Does the argument address and adequately rebut counterarguments?

A ‘yes’ answer to each of these questions should increase the reasonableness score and ‘no’ should lower it.

Note: The target audience refers to any user who is interested in the question. This includes **but is not limited to** the original poster.

Note: You should be open to seeing an argument as relevant even if it does not match your stance on the issue. Do not judge based on whether or not you agree with the author. Instead, **judge from the perspective of the target audience (see *Note 3*)**.

**Examples: Scoring reasonableness**

→ Counterarguments are in purple, Rebuttals are in blue

| Text | Score | Reason |
|---|---|---|

| | | |
|---|---|---|
| **Question:** how come Asians can't drive?<br><br>**Answer:** It's not a matter of Asians, but of how accustomed to motor vehicle operation the driver is.<br><br>A New Yorker who didn't operate a car until they were 30, and moved to California, won't be a very experienced driver, and therefore not very good at it.<br><br>Likewise, anyone who is very new to driving will seem a little clumsy. Since mass amounts of cars like we have in the Western world are still not quite commonplace in Asia, you'll see this syndrome with folks from these areas who haven't operated a car until they got here.<br><br>The question is one of experience behind the wheel, and not necessarily one of ethnicity. | **5: Very High** | The answer contributes to the resolution of the question and rebuts a counterargument. The audience would accept the answer and consider it in the larger discussion. |
| **Question:** when is it justified to fight back?<br><br>**Answer:** That depends on who your asking. Some believe its better to die before striking back, while others believe the best defense is to anticipate ones actions and strike first. I'd say do what feels best according to what you can live with based on your own conscience. How do you defend yourself? By what ever means necessary. If killing some one is not necessary then why have the blood on your hands? but if it is then so be it. And as far as gaining ones respect. You will not be respected through punishment or violence. You may gain ones fear and thus find them to be submissive to you, but respect is gained by achieving ones admiration. | **4: High** | The answer begins by addressing and rebutting counterarguments. The answer contributes to the resolution of the question and would be considered by the target audience. The target audience may or may not accept the way the argument is stated. |
| **Question:** In detail, who was the most notorious killer in history?<br><br>**Answer:** Vlad the Impaler, Prince Vlad III Dracul of Walachia, 1431--1476. Supposedly, this is the guy Bram Stoker based his novel "Dracula" on. He was called the impaler because this was his prefered method of punishment and determent. He is supposed to have executed tens of thousands of people, | **3: Medium** | The answer contributes to the resolution of the question but does not address counterarguments. The target audience may accept the way the argument is stated and may or may not consider it worthy of being mentioned in the discussion. |

| | | |
|---|---|---|
| mostly invading soldiers, though the numbers include some of his own citizens.<br><br>From the first link: By 1462, when he was deposed, he had killed between 40,000 and 100,000 people, possibly more.<br><br>I nominate Prince Dracul as the most notorious killer in history not because he killed over 100,000 people, but because he is the central figure of an entire sociocultural mythos centered around the idea of the Vampire. Every Halloween, millions of adults, adolescents, and children dress up as some variation of the vampire. A whole subgenre of fiction and entertainment is attributed to him. it is an industry that garners MegaMillions with every production ("Otherworld" for example.)<br><br>And all because of this petty princeling from the 15th centrury. | | |
| **Question:** What is the appeal of the "bad boy"?<br><br>**Answer:** They seem more exciting. But this kind of excitement is very self-destructive for the woman involved with them.<br><br>Look for your own self destructive impulses in this relatioship and try to figure out why you don't want more--such as loving kindness, stability, honesty, knowing you are with a man with solid values, knowing you are with someone who at some time will prove to be dangerous to your self esteem and will destroy what positive feelings you may have for yourself.<br><br>You don't do yourself any favors by being with a "bad boy".<br><br>They can be loving for brief periods but overall you will find your life will turn to misery and hell with a bad boy. | **2: Low** | Most of the answer is not relevant to the question and would therefore not be considered in the discussion. The author addresses a counterargument but does not adequately rebut it. |

| | | |
|---|---|---|
| **Question:** what is meant by the term "judicial activism"?<br><br>**Answer:** "Judicial activism" is code language for interpretations of laws that displease conservatives. And if George W. Bush gets his way with certain court appointments, in a while it will apply instead to displeasing liberals.<br><br>There is no real evidence of "judicial activism" in most of the historically-controversial actions of the US Supreme Court. There is evidence that outraged partisans think so. This is behind a number of attempts lately to amend the US Constitution, amendments intended to be restricive and divisive, justified on the gounds that "judicial activists" threaten the country.<br><br>Complete hogwash. | **1: Very Low** | The answer does not answer the question and therefore does not contribute to the resolution of the question. The target audience would not consider the argument in answering the question. |

**Overall:** Judge the overall quality based on your ratings of cogency, effectiveness, and reasonableness. Also, take anything outside of these three traits that influences argument quality into account.

Note: The overall score is **not** a strict average of the scores for cogency, effectiveness, and reasonableness. While the scores for these traits **should affect the overall score**, you may also consider factors not captured by these traits.

**Examples: Scoring overall**

| Text | Cogency | Effectiveness | Reasonableness | Overall |
|---|---|---|---|---|
| **Question:** how come Asians can't drive?<br><br>**Answer:** It's not a matter of Asians, but of how accustomed to motor vehicle operation the driver is.<br><br>A New Yorker who didn't operate a car until they were 30, and moved to California, won't be a very experienced driver, and therefore not very good at it. | 5: Very High | 5: Very High | 5: Very High | **5: Very High** |

| | | | | |
|---|---|---|---|---|
| Likewise, anyone who is very new to driving will seem a little clumsy. Since mass amounts of cars like we have in the Western world are still not quite commonplace in Asia, you'll see this syndrome with folks from these areas who haven't operated a car until they got here.<br><br>The question is one of experience behind the wheel, and not necessarily one of ethnicity. | | | | |
| **Question:** Disadvantages of nuclear family?<br><br>**Answer:** Compared to an extended family, A LOT. If one of the immediate family members disagree with each other on fundamental issues, that's it, the whole structure will crumble and you have a broken family and the kids will have no relatives to run to for support. I mean, they may have relatives but they will not be close enough for them to feel comfortable just knocking on their door.<br><br>Holidays are boring. You'll get cabin fever more often and... well, it's just lonely. Bigger families are more fun. | 3: Medium | 5: Very High | 3: Medium | **4: High** |
| **Question:** Is the use of the Internet making a diffrence in the way our lives are organized? What really has changed?<br><br>**Answer:** The Internet has made the world much smaller. It has changed the way we operate in our daily lives as well as in business. A recent example of how the Internet affects even the most destitute of people would be the use of notebooks and the Internet by caseworkers with Adult Protective Services in Texas. The technology they have recently introduced is awesome. A caseworker can pull up all the information needed | 4: High | 3: Medium | 3: Medium | **3: Medium** |

| | | | | |
|---|---|---|---|---|
| on a client from just about anywhere. When in the home, he/she can complete most all of the documentation. If they get lost, all they have to do is access the Internet and Yahoo Maps. It has really streamlined their work. | | | | |
| **Question:** What is the appeal of the "bad boy"?<br><br>**Answer:** They seem more exciting. But this kind of excitement is very self-destructive for the woman involved with them.<br><br>Look for your own self destructive impulses in this relatioship and try to figure out why you don't want more--such as loving kindness, stability, honesty, knowing you are with a man with solid values, knowing you are with someone who at some time will prove to be dangerous to your self esteem and will destroy what positive feelings you may have for yourself.<br><br>You don't do yourself any favors by being with a "bad boy".<br><br>They can be loving for brief periods but overall you will find your life will turn to misery and hell with a bad boy. | 1: Very Low | 3: Medium | 2: Low | **2: Low** |
| **Question:** How come we have abortion is legal but not the right to die?<br><br>**Context:** Why do we live in a society where we can't choose to end our own lives but we can choose to prohibt the life of another from existing?<br><br>Don't get me wrong, I'm not trying to start the whole pro-life or pro-chooice debate, I just want to know why we can't kill ourselves legally.... | 2: Low | 1: Very Low | 1: Very Low | **1: Very Low** |

| | | | | |
|---|---|---|---|---|
| **Answer:** Very good question!!!! My nephew was 28 wks at birth and he died, he was a whole little man. All his fingers and toes, etc. and it is legal to abort at this stage in LIFE.<br><br>And if my pet is suffering I can have them put to sleep.<br><br>But I am forced to watch a loved one die because we can't even do for them as we would a pet!!!!!! Hmmmmmm<br><br>OUR GOVERNMENT????????? | | | | |
