# Supplementary material for: Creating a Domain-diverse Corpus for Theory-based Argument Quality Assessment
Source: arXiv:2011.01589 source file (2020-11-03)
Supplement: Supplementary file 3 [file yelp_gl.pdf]

# Overview: help us judge argument quality

The goal of this task is to evaluate the argumentative quality of business reviews. You will first decide whether a given review is argumentative or not. For texts you find argumentative, you will score each of three traits: **cogency**, **effectiveness**, and **reasonableness**. You will then assign an **overall** score for the entire text snippet.

## What we provide

1. **Title:** The title of the review, which contains the name, type, and location of the business being reviewed
2. **Stars:** The author's rating of the business, which will be between **1 and 5 stars**
    - Note: The star rating for a review is the author's claim about the business. All reviews contain a claim.
3. **Review:** The full review

# Steps

1. Read the given title and review.
2. Decide if the review is argumentative.
    1. If you are unable to objectively judge the review, please choose the option that reflects why.
        - Use 'This text is not readable' only if you are not able to read and understand the example (e.g., the text is gibberish or in another language).
        - Use 'I cannot provide an objective judgment' only if your personal bias makes it impossible for you to tell if the example is argumentative and objectively score it.
    2. If you decide that the review is not argumentative, click the 'No' option and move to the next example.
    3. If you decide that the review is argumentative, click the 'Yes' option.
3. You will evaluate three traits for each text: a) cogency, b) effectiveness, and c) reasonableness.
    1. For each trait, mentally answer each of the questions presented to you with 'yes' or 'no'.
    2. Provide a score for each trait based off of your answers-- a 'yes' answer raises the score and a 'no' answer lowers it. You will score each trait on a 5-point scale:

        1: Very Low - 2: Low - 3: Medium - 4: High - 5: Very High

**Note that the number of questions is not necessarily aligned with the scale. Your answers should loosely inform your scoring.**

3. Score the overall quality of the argument last.

4. Move to the next example.

### Notes

1. The star rating for a review is the author's claim about the business. A review is argumentative if the author provides a reason for the rating they give.
2. Try to be as objective as possible. Whether or not you agree with the author should not influence whether you think the example is argumentative or how you score the example.
3. Some of the opinions stated may be offensive. If you are too offended by an example to provide an objective judgment, please choose 'I cannot provide an objective judgment' and skip to the next instance.
4. Assume the **target audience** consists of adult internet users who are open-minded, non-hostile, receptive, and generally open to being persuaded.
5. Some reviews are old and may be dated. This should not affect how you score the examples.
6. Remember to submit your work and close the window if you are going to step away from the task for a period of time.

### Tips

- After you score a trait, collapse the trait's questions by clicking on the gray box with the trait name. This makes it easier to read the passage while scoring the next trait.

# How to judge argumentativeness

You are given a Yelp review along with a title and star rating. Consider **the star rating as a claim** that the author is making about the business. You must judge whether the review provides a **reason for the star rating.**

A review should be seen as argumentative if you think that the author is arguing for the rating they gave the business. A review is not argumentative if it simply states the author's opinion about the business without any justifications for their opinion. To be considered argumentative, a review must contain a reason for the star rating.

Note: A review is argumentative if the author argues for their rating, even if they only provide one reason for their belief.

**Examples: Judging argumentativeness**

→ Claims are in orange, Justifications are in green

| Text | Argumentative? | Reason |
|---|---|---|
| **Title:** Business review: 4.0 Stars<br>Business name: Jalapeno Loco. City: Mentor.<br>Categories: Mexican, Restaurants<br><br>**Review:** Oh gosh how I miss this place.<br>I used to have dinner here every weekend with the fam before I moved. The **staff knew all of our drink and food orders by heart** and when we left they would jokingly say "see you tomorrow" but then part of me would silently think "Wait, what am I doing tomorrow... can I come back?"<br>**Cozumel chessesteak is my first pick. It's huge portions.** Have it for dinner and then take home half of it home for lunch the next day. **Chips and salsa and margaritas both are awesome and arrive quickly at the table. Friendly service.** Definitely recommend it to anyone. | **Yes** | The author supports their 4.0 Stars claim by listing justifications for giving the restaurant this rating. |
| **Title:** Business review: 1.0 Stars<br>Categories: Restaurants<br><br>**Review:** Would give 0 stars if I could. | **No** | The author does not give a reason for the 1.0 Stars rating, they just repeat their opinion. |
| **Title:** Business review: 2.0 Stars<br>Business name: Cadillac Ranch. City: Tempe.<br>Categories: Restaurants, Barbeque, Burgers, Steakhouses<br><br>**Review:** I didn't get what the concept of this place was supposed to be. Is it a country western bar, a rock and roll bar or a bar-be-que and steakhouse? One wall says saddle up, while the other says rock n roll. the place has a western design with deer antlers and guitars painted on the wall. but they kept playing love songs for music. **the food was ok, nothing real special.** i had the pulled pork sandwich, which **had a lot of grease dripping from it, and it didn't even taste as if it had been smoked. the sauce was bland and the coleslaw tasted as if had come from kfc.** | **Yes** | The author supports their 2.0 Stars claim by describing why they did not like their food. |

# How to judge argument quality

We've chosen to break the quality of an argument into the three traits listed below. You should refer to these definitions when scoring each trait.

## **Cogency:** The review includes acceptable justifications that are relevant to the author's star rating of the business. The justifications sufficiently support the author's star rating of the business.

Considering only the **individual justifications for the star rating**, answer each of the following questions before scoring cogency:

- Are the justifications for the star rating acceptable/believable?
- Are the justifications relevant to the star rating?
- Do the justifications provide enough support for the star rating?

A 'yes' answer to each of these questions should increase the cogency score and 'no' should lower it.

Note: Cogency should be scored with respect to the star rating. Consider to what degree the justifications given by the author align with their star rating of the business (i.e. a low star rating with only favorable justifications should receive a low cogency score, and vice versa).

**Examples: Scoring cogency**

→ Claims are in **orange**; Justifications are in **green**

| Text | Score | Reason |
|---|---|---|

| | | |
|---|---|---|
| **Title:** Business review: 1.0 Stars Business name: Oriental Phoenix Restaurant. City: Calgary. Categories: Vietnamese, Noodles, Desserts, Food, Chinese, Restaurants<br><br>**Review:** I would give 0 if I can. **The food here was the worst I have ever put in my mouth.** We got there, ordered, got the food in 10 mins, didn't even take us 2 mins before we decided we could not eat the served food. We ordered beef pho and sate beef pho. **The soup was luke warm and the noodles were mostly all broken into small pieces. The soup had absolutely zero flavour, it tasted like just water with salt. They don't even give you the standard bean sprouts, basil and lime**...like wtf? A small bowl of pho for $12 and no bean sprouts and lime? I felt so ripped off because **the food was inedible. WORST PHO in calgary.** | **5: Very High** | - The author supports their 1.0 Stars rating by stating multiple reasons that support this claim.<br><br>- The reasons listed are relevant, believable, and provide enough support for a 1.0 Star rating. |
| **Title:** Business review: 1.0 Stars Business name: Hipot Hot Pot Restaurant. City: Richmond Hill. Categories: Live/Raw Food, Restaurants, Hot Pot, Chinese<br><br>**Review:** Would like to give 0 star but that's not an option. **Service was the only redeeming thing this place has to offer. The food they bring to the table is of such poor quality that I would be embarrassed to feed my guests,** and to think these people charge $66 for two people for such a **sad display of stale, freezer-burned meats, and semi-rotting veggies.**<br><br>The place was dead on a friday evening should have been a red flag. My bad for staying... | **4: High** | - The 1.0 Stars rating is supported by relevant and believable justifications.<br><br>- The author could have provided more justifications to sufficiently support their conclusion. |

| | | |
|---|---|---|
| **Title:** Business review: 5.0 Stars Business name: Four Kegs Sports Bar. City: Las Vegas. Categories: American (New), American (Traditional), Sports Bars, Bars, Nightlife, Diners, Restaurants<br><br>**Review:** Ok, been back twice now and ordered their traditional Stromboli during my second visit. **The Stromboli would be the perfect child if pizza and calzones had a baby. The Stromboli is not very greasy nor is the breaking heavy. Every single bite was dreamy. I also had a taste of my friend's Philly cheesesteak and AGAIN amazing!** I love this place!!! | **3: Medium** | - The author supports their 5.0 Stars rating with acceptable and relevant justifications.<br><br>- The justifications are not sufficient to draw a conclusion. |
| **Title:** Business review: 4.0 Stars Business name: Feast Buffet. City: Henderson. Categories: Restaurants, American (Traditional), Buffets, Seafood, Barbeque, Food, American (New)<br><br>**Review:** Had never been to the GVR before, but heard it had a good breakfast buffet. I went not expecting all that much, but **it really delivered.** It doesn't offer any high end options for breakfast, but for $8.50 **it really hit the spot. The place is nice and clean, and for the money the food was really good.** Definitely will be back. | **2: Low** | - The justifications provided for the 4.0 Stars rating are vague and uninformative and are thus not acceptable.<br><br>- The author gives a relevant justification for their claim (‘The place is nice and clean…’).<br><br>- The justifications do not provide enough support for the conclusion. |
| **Title:** Business review: 3.0 Stars Business name: Crown Jewel Fine Dining. City: Scarborough. Categories: Chinese, Restaurants<br><br>**Review:** I like the fact that **we didn't have to wait for a table on a late Saturday morning.** Probably because other restaurants have deals for ordering before 11:00am. Not here. So, price conscious Chinese would come here out of necessity or convenience. We were the latter camp. **The food was average and in my opinion slightly over priced.** We entertained the set menu for dinner at just under $500, but it lacked the wow factor for that price. We'll | **1: Very Low** | - The author gives justifications that are not relevant to the claim.<br><br>- The justifications are not enough to support a 3.0 Stars rating. |

| | | |
|---|---|---|
| return someday for dinner and order off menu and see how that fares. | | |

**Effectiveness:** The way the review is presented persuades you to agree with the author, e.g. the author changed your mind or affirmed a point you already agreed with.

Answer the following questions before scoring effectiveness:

- Is the author qualified to be writing the review? Assume **yes** unless you have reason to believe the author is lying or otherwise should not be believed, i.e. they have never been a customer of the business they are reviewing.
- Does the review evoke emotions that make the audience more likely to agree with the author?
- Does the author's language make it easy for you to understand what they are arguing for or against? Consider if the author uses grammatically correct and unambiguous language, avoids unnecessary complexity, and stays on topic.
- Is the review and its delivery appropriate for an online forum? (Note: Offensive language should always be considered inappropriate.)
- Does the author present the review in an order that makes sense?

A 'yes' answer to each of these questions should increase the effectiveness score and 'no' should lower it.

**Examples: Scoring effectiveness**

| Text | Score | Reason |
|---|---|---|

| | | |
|---|---|---|
| **Title:** Business review: 5.0 Stars Business name: Thai Basil. City: Richmond Hill. Categories: Pan Asian, Thai, Restaurants<br><br>**Review:** Thai Basil, coming from a chef this is indeed a Michelin star quality establishment. The food is top notch, you won't find anything like it in the GTA. Green curry is unlike anything I've had before. To top it off the service is far too good to be true. No matter how many times I try to let my cup run dry it never happens. | **5: Very High** | - The author is explicitly qualified to write the review.<br><br>- The author's language makes it easy to understand their argument.<br><br>- The delivery is appropriate. |
| **Title:** Business review: 5.0 Stars Business name: B&M Bar-b-que. City: Cleveland. Categories: Restaurants, Barbeque<br><br>**Review:** When you want some good 'ol 'down home' bar-b-que, then you need to head on in to B&M! I go to the E. 105th, E. 152nd, and the one Bellaire on the westside. This is probably the best bar-b-que and soul food in Cleveland! The customer service is excellent on the westside. My favorite dinner is the chicken wings. Can't get enough! They are seasoned, battered fried to perfection, and the sauce is good. Try 'em you won't be disappointed. | **4: High** | - The review is easy to understand and well organized.<br><br>- The author's use of creative spelling evokes emotions that make the review more agreeable.<br><br>- The author's spelling is overly complex. |
| **Title:** Business review: 2.0 Stars Business name: Cadillac Ranch. City: Tempe. Categories: Restaurants, Barbeque, Burgers, Steakhouses<br><br>**Review:** I didn't get what the concept of this place was supposed to be. Is it a country western bar, a rock and roll bar or a bar-be-que and steakhouse? One wall says saddle up, while the other says rock n roll. the place has a western design with deer antlers and guitars painted on the wall. but they kept playing love songs for music. the food was ok, nothing real special. i had the pulled pork | **3: Medium** | - The author's language does not make it easy to understand what they are arguing for in that they do not stay on topic.<br><br>- The review is appropriate for an online forum.<br><br>- The use of humor evokes emotions that make the review more agreeable. |

| | | |
|---|---|---|
| sandwich, which had a lot of grease dripping from it, and it didn't even taste as if it had been smoked. the sauce was bland and the coleslaw tasted as if had come from kfc. | | |
| **Title:** Business review: 1.0 Stars Business name: Ah-So Sushi & Steak. City: Peoria. Categories: Japanese, Sushi Bars, Restaurants, Steakhouses<br><br>**Review:** I went to this ahso a year ago and got shitty slow service. The same people I went with we all went again yesterday. The service is super slow my entree I got was cold. My entire family is never going here again also my friend who was behind us had problems and isn't coming again either. This restaurant is overpriced An the service should make up for that but don't. | **2: Low** | - The review is presented in an order that does not make sense.<br><br>- The author does not evoke any emotions.<br><br>- The author does not use clear language. |
| **Title:** Business review: 1.0 Stars Business name: Hakkasan Nightclub. City: Las Vegas. Categories: Nightlife, Chinese, Lounges, Cantonese, Bars, Dance Clubs, Restaurants<br><br>**Review:** I am severely disabled with my feet. Because of this I have to wear light weighted sportive shoes. I weared brand new Pure black Nike ID sneakers with cool red latches. I payed for entrance with my wife 50 dollars and was still waiting in line, after 15 minutes a bouncer throwed me out of the line and sayed to me my shoes are not correct and I can't go in. i asked, why he not also puts out of the line the probably 20% other people in line wearing sneakers - he was only smiling arrogant down on me! What a f....ing place is this, never happened to me and my wife before! I read in other reviews: If you buy for 7.500 dollar up an VIP table you can wear what you want, hat, tshirt no problem. They put 3.000 dollar champagne bottles on your bill you never ordered and other things... Best | **1: Very Low** | - The author does not use clear language.<br><br>- The review is presented in a confusing order.<br><br>- The author's language in somewhat inappropriate for an online forum. |

| | | |
|---|---|---|
| electronic music club in the world? Not with this employees! | | |

**Reasonableness:** The review sufficiently contributes to the discussion about the quality of the business in a way that is acceptable to the target audience.

Considering the **entire review**, answer the following questions before scoring reasonableness:

- Would the target audience accept the review and the way it is stated?
  - Note: The star rating can be considered as part of how the review is stated. Consider if the audience would judge the star rating as reasonable given the review.
- Would the target audience judge the argument as worthy of being mentioned in the larger discussion?
- Does the argument contribute to the resolution of the given issue, which is the quality of the business? Does it provide information that helps the audience arrive at a conclusion?
- Does the review address and adequately rebut counterarguments?

A ‘yes’ answer to each of these questions should increase the reasonableness score and ‘no’ should lower it.

**Note:** You should be open to seeing an argument as relevant even if it does not match your stance on the issue. Do not judge based on whether or not you agree with the author. Instead, **judge from the perspective of the target audience (see *Note 4*)**.

How to judge counterarguments

In the context of reviews, the following should be considered counterarguments:

→ Counterarguments are in **purple**; Rebuttals are in **blue**

1. Addressing and rebutting the **viewpoints of other reviews**

   “Everyone says that **the pizza crust is too thin here** **but that’s authentic!**”

2. Addressing and rebutting points that **discredit the author’s rating**
   a. Bringing up unfavorable points in a favorable review:

      “I love everything about this restaurant but **the service could be better.** **It was really busy, though.**”

b. Bringing up favorable points in an unfavorable review

“I did not enjoy my time here… at least **the atmosphere was interesting.** But **they need to update the old furniture!**”

**Examples: Scoring reasonableness**

→ Counterarguments are in **purple**; Rebuttals are in **blue**

| Text | Score | Reason |
|---|---|---|
| **Title:** Business review: 3.0 Stars Business name: P.J. Clarke's New York Chophouse. City: Las Vegas. Categories: Steakhouses, Gastropubs, Seafood, American (New), Venues & Event Spaces, Beer, Wine & Spirits, Restaurants, Food, Event Planning & Services<br><br>**Review:** P.J.s was Ok - **over-priced for the quality of food, but that is about standard for the strip I guess.** My wife, a couple friends and I stopped in for a quick bite before heading out of town. In general the food is pretty good, but there are some execution problems. French fries where over done, Caprese salad was drowned in vinaigrette, and the fish and chips were drowned in grease. The other entrees we got were fine - I got salmon which was very well cooked and my two friends got a burger, and mini-tacos (**I have never seen tacos that small**...**but he reported they were good**)<br><br>The atmosphere is nice - close and intimate.<br><br>Overall, I would recommend passing on P.J.s | **5: Very High** | - The target audience would accept the review and consider it worthy of being mentioned.<br><br>- The review helps the audience arrive at a conclusion about the business.<br><br>- The review addresses and adequately rebuts counterarguments. |

| | | |
|---|---|---|
| **Title:** Business review: 4.0 Stars Business name: Frankie's Italian Cuisine. City: North Olmsted. Categories: Restaurants, Italian, Pizza<br><br>**Review:** I was very skeptical about this place but I have to admit it - it's good stuff. Regardless of **dated interior and scarce veggies in the salad** ( after all **you don't come to restaurant to admire new carpet or count cucumbers in your salad**), it's worth paying for.<br><br>Highlights of the dinner were house dressing ( very evolved version of poppy seed one) and chicken Tosca. The latter was simply divine-melting-in-your-mouth experience. Calamari were also good, **maybe a tad over-fried**, but again, **who cares about that when you were given more than full glass of excellent malbec to wash it down?**<br><br>On my own scale of authenticity, it was 8 out of 10. And how they still haven't taken Olive Garden down the street out of business, I'll never know. | **4: High** | - The target audience would accept the review and consider it worthy of being mentioned.<br><br>- The review helps the audience arrive at a conclusion about the business.<br><br>- The review addresses counterarguments but may or may not adequately rebut them. |
| **Title:** Business review: 5.0 Stars Business name: Malabar. City: Charlotte. Categories: Spanish, Restaurants<br><br>**Review:** If you're in the mood for tapas, stop by recently opened Malabar. I was there for the first time with a party of 14 that the manager graciously made space for. We all walked away super happy with what we ordered whether we opted for tapas or entrees. The wine by the glass is also yum no matter what you order. One of the tapas I had was the asparagus omelet and I cannot get the taste out of my mind - it was that good. One thing I will say, is that I feel like **I have already tasted the whole menu for what is available for vegetarians -** | **3: Medium** | - The target audience would judge the review as worthy of being mentioned.<br><br>- The review helps the audience arrive at a conclusion about the business.<br><br>- The author addresses a counterargument but does not rebut it. |

| | | |
|---|---|---|
| **would be good to have special tapas to get me to come back and try something new!** | | |
| **Title:** Business review: 4.0 Stars Business name: Feast Buffet. City: Henderson. Categories: Restaurants, American (Traditional), Buffets, Seafood, Barbeque, Food, American (New)<br><br>**Review:** Had never been to the GVR before, but heard it had a good breakfast buffet. **I went not expecting all that much, but it really delivered. It doesn't offer any high end options for breakfast, but for $8.50 it really hit the spot.** The place is nice and clean, and for the money the food was really good. Definitely will be back. | **2: Low** | - The audience may or may not consider the review as worthy of being mentioned.<br><br>- The review only slightly helps the audience arrive at a conclusion.<br><br>- The author addresses counterarguments but does not rebut them adequately. |
| **Title:** Business review: 2.0 Stars Business name: Kabuki Japanese Restaurant. City: Las Vegas. Categories: Sushi Bars, Restaurants, Asian Fusion, Japanese<br><br>**Review:** Now I'm no Daniel LaRusso with a chopstick, but I have never had so many pieces of sushi crumble when I tried to eat them. I have only been too a handful of sushi places, but his has to be my least favorite of them all.<br><br>Maybe it's because someone decided to order for the whole table and I wasn't able to get what I wanted or the fact that everything that came seemed thrown together what ever it was I didn't have a good experience here. | **1: Very Low** | - The audience would not consider the review as worthy of being mentioned.<br><br>- The review does not contribute to the discussion.<br><br>- The author does not address counterarguments. |

**Overall:** Judge the overall quality based on your ratings of cogency, effectiveness, and reasonableness. Also, take anything outside of these three traits that influences argument quality into account.

Note: The overall score is **not** a strict average of the scores for cogency, effectiveness, and reasonableness. While the scores for these traits should affect the overall score, you may also consider factors not captured by these traits.

**Examples: Scoring overall**

| Text | Cogency | Effectiveness | Reasonableness | Overall |
|---|---|---|---|---|
| **Title:** Business review: 4.0 Stars Business name: Frankie's Italian Cuisine. City: North Olmsted. Categories: Restaurants, Italian, Pizza<br><br>**Review:** I was very skeptical about this place but I have to admit it - it's good stuff. Regardless of dated interior and scarce veggies in the salad ( after all you don't come to restaurant to admire new carpet or count cucumbers in your salad), it's worth paying for.<br><br>Highlights of the dinner were house dressing ( very evolved version of poppy seed one) and chicken Tosca. The latter was simply divine-melting-in-your-mouth experience. Calamari were also good, maybe a tad over-fried, but again, who cares about that when you were given more than full glass of excellent malbec to wash it down?<br><br>On my own scale of authenticity, it was 8 out of 10. And how they still haven't taken Olive Garden | 5: Very High | 5: Very High | 4: High | **5: Very High** |

| | | | | |
|---|---|---|---|---|
| down the street out of business, I'll never know. | | | | |
| **Title:** Business review: 3.0 Stars Business name: P.J. Clarke's New York Chophouse. City: Las Vegas. Categories: Steakhouses, Gastropubs, Seafood, American (New), Venues & Event Spaces, Beer, Wine & Spirits, Restaurants, Food, Event Planning & Services<br><br>**Review:** P.J.s was Ok - over-priced for the quality of food, but that is about standard for the strip I guess. My wife, a couple friends and I stopped in for a quick bite before heading out of town. In general the food is pretty good, but there are some execution problems. French fries where over done, Caprese salad was drowned in vinaigrette, and the fish and chips were drowned in grease. The other entrees we got were fine - I got salmon which was very well cooked and my two friends got a burger, and mini-tacos (I have never seen tacos that small...but he reported they were good)<br><br>The atmosphere is nice - close and intimate.<br><br>Overall, I would recommend passing on P.J.s | 4: High | 4: High | 5: Very High | **4: High** |

| | | | | |
|---|---|---|---|---|
| **Title:** Business review: 5.0 Stars Business name: B&M Bar-b-que. City: Cleveland. Categories: Restaurants, Barbeque<br><br>**Review:** When you want some good 'ol 'down home' bar-b-que, then you need to head on in to B&M! I go to the E. 105th, E. 152nd, and the one Bellaire on the westside. This is probably the best bar-b-que and soul food in Cleveland! The customer service is excellent on the westside. My favorite dinner is the chicken wings. Can't get enough! They are seasoned, battered fried to perfection, and the sauce is good. Try 'em you won't be disappointed. | 2: Low | 4: High | 3: Medium | **3: Medium** |
| **Title:** Business review: 2.0 Stars Business name: Char-Grill. City: Davidson. Categories: American (Traditional), Food, Restaurants, Burgers<br><br>**Review:** First off, let me say I believe Five Guys has ruined me for any other burger place.<br><br>I didn't like Char-Grill, I felt the burger was dry, even after I had chili put on mine and the fries were just ok. I think I could have got the same thing at a fast food place for .99 cents. I probably won't go back, unless someone else suggests it... maybe. | 3: Medium | 2: Low | 2: Low | **2: Low** |
| **Title:** Business review: 2.0 Stars Business name: Kabuki Japanese Restaurant. City: Las Vegas. Categories: Sushi Bars, Restaurants, Asian Fusion, Japanese | 1: Very Low | 2: Low | 1: Very Low | **1: Very Low** |

| | | | | |
|---|---|---|---|---|
| **Review:** Now I'm no Daniel LaRusso with a chopstick, but I have never had so many pieces of sushi crumble when I tried to eat them. I have only been too a handful of sushi places, but his has to be my least favorite of them all.<br><br>Maybe it's because someone decided to order for the whole table and I wasn't able to get what I wanted or the fact that everything that came seemed thrown together what ever it was I didn't have a good experience here. | | | | |

## Extra examples (if needed)

**Title:** Business review: 2.0 Stars Business name: Molson Pub. City: Toronto. Categories: Food, Bars, Coffee & Tea, Nightlife, Restaurants, Pubs

**Review:** In Pearson's Air Canada international terminal, meal options are slim (bad sushi, Pizza Pizza, bland sandwiches, etc.). If you want a place to sit down and drink beer, then Molson Pub is your place. As for the food, I wasn't too satisfied when I went last week.

I ordered the Montreal Smoke Meat Sandwich w/ Poutine ($13.50). It comically came with a Canadian flag toothpicked into the sandwich (see picture). The food was subpar and not cheap, but then again what do you expect from airport food?

**Title:** "Business review: 5.0 Stars
Business name: Creek Side Taco Shack. City: Queen Creek. Categories: Restaurants, Mexican, Tacos"
**Stars:** 5
**Review:** This place is not 5 stars, but with a few tweaks, it could be. I am giving it 5 stars so that the ranking on yelp doesn't go any lower. I hope management is reading these reviews as most people are spot on.  Needs: better customer service training for your staff, better lighting for night time sports, additional seating. This stuff is easy, but will be the demise if not corrected.
